# Supplementary material for: A phase-field approach for modeling equilibrium solute segregation at the interphase boundary in binary alloys
Source: arXiv:1910.05606 source file (2019-10-27)
Supplement: Supplementary file 2 [file appendix.tex]

\section{Phase-Field Profile, WBM model}

\begin{align} \label{apeq:eq_phi}
    \left. \frac{\partial f(c_e,\phi_e)}{\partial \phi_e} \right. + W(c_e)\frac{dg}{d\phi_e} - \epsilon^2  \frac{d^2 \phi_e}{d x^2}  = 0
\end{align}

\begin{align} \label{apeq:eq_phi_diff}
    \epsilon^2  \frac{d^2 \phi_e}{d x^2}  = \left[f_\beta(c_e) - f_\alpha(c_e)\right]\frac{dh}{d\phi_e} + W(c_e)\frac{dg}{d\phi_e}
\end{align}

Multiplying both sides with ${d\phi_e}/{dx}$ and integrating

\begin{align} \label{apeq:eq_phi_int}
    \frac{\epsilon^2}{2} \left(\frac{d\phi_e}{dx}\right)^2 = \int_0^{\phi_e} \left[f_\beta(c_e) - f_\alpha(c_e)\right]\frac{dh}{d\phi_e} d\phi_e + \int_0^{\phi_e} W(c_e)\frac{dg}{d\phi_e} d\phi_e
\end{align}

where, $c_e = c_e(\phi_e(x))$. Integration by parts both terms on right hand side

\begin{align} \label{apeq:eq_phi_byparts} \nonumber
    \frac{\epsilon^2}{2} \left(\frac{d\phi_e}{dx}\right)^2 =& \left[f_\beta(c_e) - f_\alpha(c_e)\right]h(\phi_e) - \int_{c_e^\alpha}^{c_e} \left(\frac{d f_\beta}{dc_e} - \frac{d f_\alpha}{d c_e} \right)h(\phi_e) dc_e \\
    &+ W(c_e)g(\phi_e) - \int_{c_e^\alpha}^{c_e} \frac{\partial W}{\partial c_e} g(\phi_e) dc_e
\end{align}

The terms within the integral can be combined, and using the steady-state relation for concentration (Eq. \ref{eq:steady-state_c_seg}), can be expressed as

\begin{align} \label{apeq:eq_phi_byparts_subst}
    \frac{\epsilon^2}{2} \left(\frac{d\phi_e}{dx}\right)^2 =& \left[f_\beta(c_e) - f_\alpha(c_e)\right]h(\phi_e) + W(c_e)g(\phi_e) - \int_{c_e^\alpha}^{c_e} \left(\left.\frac{\partial f_\alpha}{\partial c_e}\right|_{c_e^\alpha} - \frac{\partial f_\alpha}{\partial c_e}\right) dc_e
\end{align}

% \begin{align}
%     \frac{\epsilon^2}{2} \left(\frac{d\phi_e}{dx}\right)^2 = \left. \frac{\partial f}{\partial c} \right|_{c_e} = \mu_c^e \textrm{ (const.)}
% \end{align}
Equation for the equilibrium phase field $\phi_e$

\begin{align} \label{apeq:eq_phi_profile}
    \frac{\epsilon^2}{2} \left(\frac{d\phi_e}{dx}\right)^2 &= W(c_e)g(\phi_e) + f(c_e,\phi_e) - f_\alpha(c_e^\alpha) - \left.\frac{\partial f_\alpha}{\partial c_e}\right|_{c_e^\alpha}(c_e - c_e^\alpha) \\
    &= W(c_e)g(\phi_e) + G(c_e,\phi_e)
\end{align}

% \section{Interface Segregation}

% \begin{align}
%     \left. \frac{\partial f(c_e,\phi_e)}{\partial c_e} \right. = \left.\frac{\partial f_\alpha}{\partial c}\right|_{c_e^\alpha} = \mu_c^e \textrm{ (const.)}
% \end{align}

% \begin{align*}
%      \frac{c_e(x)}{1-c_e(x)} = \frac{c_e^\alpha}{1-c_e^\alpha} \exp\left(\frac{\Delta H_{seg}}{RT/V_{m}}\right)
% \end{align*}

% where,
% \begin{align*}
%     \Delta H_{seg} &= G_\alpha^B - G^B(\phi_e) - G_\alpha^A - G^A(\phi_e) + \left[\Omega_\alpha - \Omega(\phi_e)\right](1-2c_e)  
% \end{align*}

\section{Interface Energy, WBM Model}

The interfacial energy is defined as \cite{mcfadden2002gibbs,wheeler1992phase,lupis1983chemical,provatas2011phase}

\begin{align} \label{apeq:gamma_lit}
    \gamma = (F-F_{o}) - \Gamma_B \left.\frac{\partial f_\alpha}{\partial c}\right|_{c_e^\alpha}
\end{align}

where, $F$ is given by Eq. \ref{eq:F_total}, $\Gamma_B$ is given by Eq. \ref{eq:excess_reln}. The second term assumes $\Gamma_A = -\Gamma_B$, which holds when the molar volumes of components $A$ and $B$ are equal. $F_{o}$ is the total free energy of the sharp-interface reference system defined by

\begin{align}
    F_{o} = \int_{-L}^{0} f_\alpha(c_e^\alpha) dx + \int_{0}^{+L} f_\beta(c_e^\beta) dx
\end{align}

Substituting relations for $F$, $F_{o}$ and $\Gamma_B$ gives
% 

% \begin{align}
%     \gamma =& \int_{-L}^{0} \left[\frac{\epsilon^2}{2}\left(\frac{d\phi_e}{dx}\right)^2 + f(c_e,\phi_e) - f_\alpha(c_e^\alpha) - \mu_c^e (c_e - c_e^\alpha) \right] dx \\
%     &+ \int_{0}^{+L} \left[\frac{\epsilon^2}{2}\left(\frac{d\phi_e}{dx}\right)^2 + f(c_e,\phi_e) - f_\beta(c_e^\beta) - \mu_c^e (c_e - c_e^\beta) \right] dx
% \end{align}

\begin{align}
    \gamma =& \int_{-L}^{+L} \left[\frac{\epsilon^2}{2}\left(\frac{d\phi_e}{dx}\right)^2 + f(c_e,\phi_e) - \mu_c^e c_e \right] dx \\
    &- \int_{-L}^{0} \left[f_\alpha(c_e^\alpha) - \mu_c^e c_e^\alpha \right] dx - \int_{0}^{+L} \left[f_\beta(c_e^\beta) - \mu_c^e c_e^\beta \right] dx
\end{align}

Using the equation for equilibrium phase-field (Eq. \ref{apeq:eq_phi_profile}) and the common tangent relation (Eq. \ref{eq:common_tgt}) yields

% \begin{align} \label{apeq:deltaF_lit}
%     \Delta F =& \int_{-L}^{+L} \left[f(c_e,\phi_e)+\frac{\epsilon^2}{2}\left(\frac{d\phi_e}{dx}\right)^2 \right] dx - \int_{-L}^{0} f_\alpha(c_e^\alpha) dx - \int_{0}^{+L} f_\beta(c_e^\beta) dx
% \end{align}

\begin{align} \label{apeq:gamma_int}
    \gamma = \epsilon^2 \int_{-L}^{L} \left(\frac{d\phi_e}{dx}\right)^2 dx
    = \epsilon^2 \int_{0}^{1} \left(\frac{d\phi_e}{dx}\right) d\phi_e
\end{align}

Interface excess regular solution parameters:

\begin{align}
    \Omega_{xs} = \int_{-L}^{+L} \Omega\left(\phi_e(x)\right) \, dx - \int_{-L}^{0} \Omega_\alpha \, dx - \int_{0}^{+L} \Omega_\beta \, dx
\end{align}

\begin{align}
    G^A_{xs} = \int_{-L}^{+L} G^A\left(\phi_e(x)\right) \, dx - \int_{-L}^{0} G^A_\alpha \, dx - \int_{0}^{+L} G^A_\beta \, dx
\end{align}

\begin{align}
    G^B_{xs} = \int_{-L}^{+L} G^B\left(\phi_e(x)\right) \, dx - \int_{-L}^{0} G^B_\alpha \, dx - \int_{0}^{+L} G^B_\beta \, dx
\end{align}
