# Supplementary material for: A phase-field approach for modeling equilibrium solute segregation at the interphase boundary in binary alloys
Source: arXiv:1910.05606 source file (2019-10-27)
Supplement: Supplementary file 3 [file appendix_interface_thermodynamics.tex]

\section{Interface Thermodynamics}

For the entire system $[-l,l]$ which completely includes the inhomogeneous interfacial region
\begin{flalign}
    d\gamma = -[S]dT + VdP - [N_A]d\mu_A - [N_B]d\mu_B &&
\end{flalign}
where $[S] = {S_l}/{A_i} = \int_{-l}^{l} s(x) dx$, $[V] = {V_l}/{A_i} = \int_{-l}^{l} dx$, $[N_k] = N_k/A_i = \int_{-l}^{l} \rho_k(x) dx $.

Gibbs-Duhem relations for bulk phases:
\begin{flalign}
    0 = - S^m dT + V^m dP - N_A^m d\mu_A - N_B^m d\mu_B &&
\end{flalign}
\begin{flalign}
    0 = - S^p dT + V^p dP - N_A^p d\mu_A - N_B^p d\mu_B &&
\end{flalign}

Using Cramer's rule,
\begin{flalign}
    d\gamma = -[S/XY] dT + [V/XY] dP - [N_A/XY] d\mu_A - [N_B/XY] d\mu_B &&
\end{flalign}
where,
\begin{flalign}
    [Z/XY] = \frac{|[Z] X^m Y^p|}{|X^m Y^p|} = \frac{\begin{vmatrix}
        [Z] & [X] & [Y] \\
        S^m & X^m & Y^m \\
        S^p & X^p & Y^p
    \end{vmatrix}}{
    \begin{vmatrix}
        X^m & Y^m \\
        X^p & Y^p
    \end{vmatrix}} &&
\end{flalign}
Choosing ${X,Y}={V,N_A}$, variation in $\gamma$ in terms of the independent quantities $dT$ and $d\mu_B$ is given by
\begin{flalign}
    d\gamma = -[S/VN_A]dT - [N_B/VN_A]d\mu_B &&
\end{flalign}
where
\begin{flalign}
    [S/VN_A] = \int_{-l}^{l} \left[(s(x) - s^m) - \frac{(s^p-s^m)}{(c_A^p-c_A^m)} (c_A(x)-c_A^m) \right] dx &&
\end{flalign}
\begin{flalign}
    [N_B/VN_A] = \rho_o \int_{-l}^{l} \left[(c_B(x) - c_B^m) - \frac{(c_B^p-c_B^m)}{(c_A^p-c_A^m)} (c_A(x)-c_A^m) \right] dx &&
\end{flalign}
The constraint $c_A(x)+c_B(x)=1$ results in $[N_B/VN_A]=0$ and
\begin{flalign}
    [S/VN_A] = \int_{-l}^{l} \left[(s(x) - s^m) - \frac{(s^p-s^m)}{(c_B^p-c_B^m)} (c_B(x)-c_B^m) \right] dx &&
\end{flalign}
Therefore,
\begin{flalign}
    \frac{d\gamma}{dT} = -[S/VN_A] = - [S/VN_B] = - [S/VC] &&
\end{flalign}
